# Supplementary material for: OATS: Opinion Aspect Target Sentiment Quadruple Extraction Dataset for Aspect-Based Sentiment Analysis
Source: arXiv:2309.13297 source file (2024-03-06)
Supplement: Supplementary file 1 [file 7-Appendix.tex]

\section{Appendix: OATS Corpus Properties}
\label{Sec: Properties}
    We set the following properties or requirements for the corpus to make it ideal for future works:
    \begin{itemize}
        \item \textbf{Each review should have both sentence-level and review/text-level annotations}: The goal of this dataset is not just to provide some sentence-level aspect-related information but rather include review-level or text-level annotations as well. 
        That is, given a text, we should do the following two steps:
            \begin{enumerate}
                \item Take each individual sentence in the text and extract all the aspect terms and opinion phrases followed by categorizing them into aspect categories and sentiment polarity, respectively, forming a quadruple. Each sentence can have multiple such quadruples. 
                \item After getting the quadruples from all the sentences, take the unique aspect categories from them and assign the sentiment polarity (positive, negative, neutral, or conflict) that is dominant from the sentiment assigned in those quadruples. If the positive and negative sentiments are equally strong, assign a \textit{conflict} opinion polarity to that aspect category. 
            \end{enumerate}
        \item \textbf{As little ambiguity as possible and easily understandable aspect categories:} To avoid ambiguity when assigning aspect categories to a review or a sentence, one of the lessons learned from prior datasets is that those aspect categories should be nearly mutually exclusive. Additionally, the aspect categories should be relevant to the domain and easily comprehended by anyone. 
        \item \textbf{Inclusion of both implicit targets and implicit opinions}: As we mentioned in Section \ref{Sec: Introduction}, there may be cases where the opinion target or the opinion expression could be implicit. We include both those cases and assign \texttt{NULL} to that element in the quadruple. If both are implicit, both the elements will be marked as \texttt{NULL}. 
        \item \textbf{Start and End indices of the text spans should be provided}: To facilitate diverse formulations of ABSA, we aim to provide the start and end indices of the opinion target and opinion phrase annotations for each quadruple. This could be helpful for question-answering type formulations. 
        \item \textbf{Reviews should have an adequate number of sentences}: Each review in the dataset should have a minimum number of sentences that will help differentiate the sentence-level and review/text-level tasks of ABSA. 
        If reviews are one to two sentences long, there is a chance that review-level ABSA may degenerate to sentence-level ABSA achieving good performance with the sentence-level models itself. 
        Therefore, we chose to keep only those reviews that are at least four to eight sentences long. 
    \end{itemize}

\section{Appendix: Defining Fine-Grained Annotations}
\label{Sec: Fine-Grained Annotations}
    With the above requirements and properties in place, we began our process of finding aspect categories for each domain. 
    For the TripAdvisor Hotel reviews, we chose to use the aspect categories defined in the shared task organized by \cite{16-dataset}, where there is a small Arabic dataset for hotel reviews. Eight entities and seven attributes result in 26 Entity\#Attribute pairs as shown in Table \ref{tab: Hotels-EA-pairs}. 
    We followed the below steps to define the several entities and attributes that form an aspect category for Coursera and amazon fine foods domains:
    \begin{itemize}
        \item From the entire review dataset, we generated a list of frequently occurring words and phrases. 
        \item From that list, we filtered all the nouns and noun phrases. Then, we applied a clustering algorithm on the nouns and noun phrases with the number of clusters varying from three to eight. 
        \item From those clusters, we manually verified the intra-cluster word synonymity and relationships that led to identifying the correct number of clusters. 
        \item From those clusters, we came up with the most generic entity-attribute pairs that could sufficiently represent the cluster. 
    \end{itemize}
    Then, we selected a pool of 2000 reviews from the entire dataset with the following constraints:
    \begin{itemize}
        \item There should be at least 4 sentences in each review
        \item Each review should have at least 2 distinct aspect categories
    \end{itemize}
    We used a Siamese-BERT model \cite{Siamese-BERT} to determine whether a review has at least two of the defined aspect categories in the domain. 
    Specifically, we gave the review and the sentence ``\textit{This review mentioned about [aspect category]}'' as an input to the model. If the similarity score is greater than 0.75 for more than two aspect categories, we take that review for the annotation procedure. 
    We present the entity-attribute pairs for each domain in Tables \ref{tab: Amazon-EA-pairs}, \ref{tab: Coursera-EA-pairs}, and \ref{tab: Hotels-EA-pairs}.

    \begin{table*}[!h]
        \centering
        \resizebox{0.9\textwidth}{!}{%
        \begin{tabular}{|l|c|c|c|c|c|c|c|c|}
        \hline
        \textbf{Entity/Attribute}                & GENERAL & PRICES & DESIGN\&FEATURES & CLEANLINESS & COMFORT & QUALITY & STYLE\&OPTIONS & MISCELLANEOUS \\ \hline
        HOTEL           & \cmark & \cmark & \cmark & \cmark & \cmark & \cmark  & \xmark  & \cmark \\ \hline
        ROOMS           & \cmark & \cmark & \cmark & \cmark & \cmark & \cmark  & \xmark  & \cmark  \\ \hline
        ROOM\_AMENITIES & \cmark & \cmark  & \cmark & \cmark & \cmark  & \cmark & \xmark  & \cmark  \\ \hline
        FACILITIES      & \cmark & \cmark & \cmark & \cmark & \cmark & \cmark & \xmark  & \cmark  \\ \hline
        SERVICE         & \cmark & \xmark  & \xmark  & \xmark  & \xmark  & \xmark  & \xmark  & \xmark  \\ \hline
        LOCATION        & \cmark & \xmark  & \xmark  & \xmark  & \xmark  & \xmark  & \xmark  & \xmark  \\ \hline
        FOOD\&DRINKS    & \xmark  & \cmark & \xmark  & \xmark  & \xmark  & \cmark & \cmark & \cmark  \\ \hline
        \end{tabular}%
        }
        \caption{Hotels domain possible Entity Attribute pairs}
        \label{tab: Hotels-EA-pairs}
    \end{table*}

    \begin{table*}[!h]
        \centering
        \resizebox{0.9\textwidth}{!}{%
        \begin{tabular}{|l|c|c|c|c|c|c|c|c|}
        \hline
        \textbf{Entity/Attribute}             & GENERAL & QUALITY & COMPREHENSIVENESS & RELATABILITY & WORKLOAD & RESPONSE & VALUE & QUANTITY \\ \hline
        PRESENTATION & \xmark      & \cmark     & \cmark               & \cmark          & \cmark      & \xmark       & \xmark    & \xmark      \\ \hline
        ASSIGNMENTS  & \xmark      & \cmark     & \cmark               & \cmark          & \cmark      & \xmark       & \xmark    & \cmark     \\ \hline
        MATERIAL     & \xmark      & \cmark     & \cmark               & \cmark          & \cmark      & \xmark       & \xmark    & \cmark     \\ \hline
        GRADES       & \cmark     & \xmark      & \xmark                & \xmark           & \xmark       & \xmark       & \xmark    & \xmark      \\ \hline
        FACULTY      & \cmark     & \xmark      & \cmark               & \cmark          & \xmark       & \cmark      & \cmark   & \xmark      \\ \hline
        COURSE       & \cmark     & \cmark     & \cmark               & \cmark          & \cmark      & \xmark       & \cmark   & \xmark      \\ \hline
        \end{tabular}%
        }
        \caption{Coursera courses domain possible Entity Attribute pairs}
        \label{tab: Coursera-EA-pairs}
    \end{table*}

    \begin{table*}[!h]
        \centering
        \resizebox{0.8\textwidth}{!}{%
        \begin{tabular}{|l|l|l|l|l|l|l|}
        \hline
        \textbf{Entity/Attribute}         & GENERAL & QUALITY & STYLE\_OPTIONS & PRICES & DELIVERY & AVAILABILITY \\ \hline
        FOOD     & \cmark     &\cmark     & \cmark            & \cmark    & \xmark       & \xmark           \\ \hline
        SHIPMENT & \xmark     &\cmark     & \xmark             & \cmark    & \cmark      & \xmark           \\ \hline
        AMAZON   & \xmark     &\xmark      & \xmark             & \cmark    & \xmark       & \cmark          \\ \hline
        \end{tabular}%
        }
        \caption{Amazon Fine Foods domain possible Entity Attribute pairs}
        \label{tab: Amazon-EA-pairs}
    \end{table*}

    \begin{figure}[!h]
        \centering
        \includegraphics[width=\linewidth]{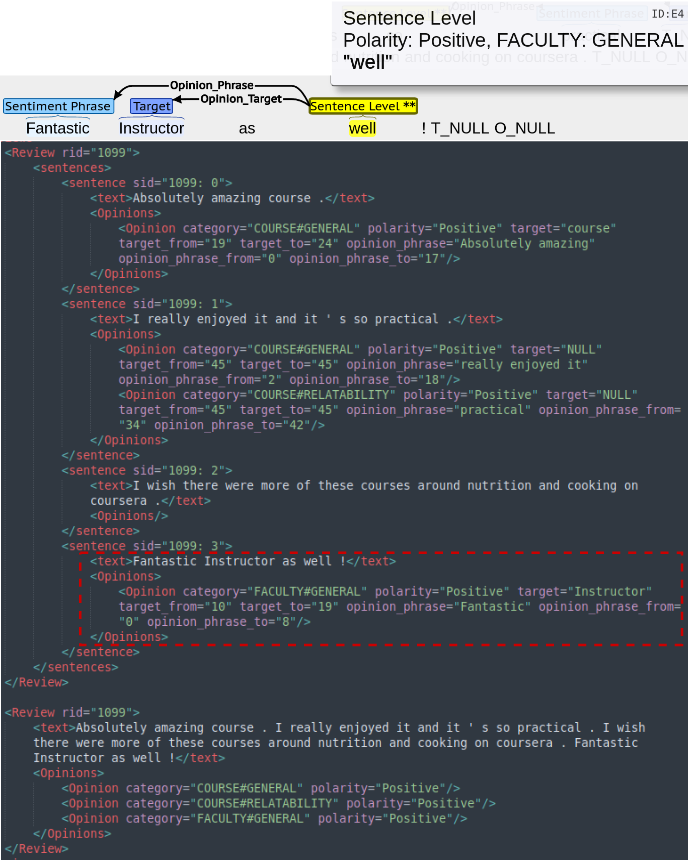}
        \caption{Example of an opinion quadruple from a sentence in the Coursera domain in BRAT format and the final XML format of the sentence-level and review-level annotations of a review}
        \label{fig: brat}
    \end{figure}

\section{Appendix: Inter-Annotator Agreement}
\label{Sec: Appendix-IAA}
